# Supplementary material for: Predicting Scores of Medical Imaging Segmentation Methods with Meta-Learning
Source: arXiv:2005.08869 source file (2020-05-08)
Supplement: Supplementary file 1 [file supplementaryMaterial.tex]

\section{Supplementary material}

\subsection{Statistical metafeatures}
List of 33 statistical features used to compose the statistical metafeatures.
\setcounter{table}{0}

\label{appendix:stat}
\begin{table}[!h]
\centering
\resizebox{\textwidth/3}{!}{
\begin{tabular}{l}
\hlineB{4}
\textbf{Statistical metafeatures}\\\hlineB{4}
Number of instances\\\hline
Voxel value M\\\hline
Voxel value STD\\\hline
Voxel value CVAR\\\hline
Skew M\\\hline
STD\\\hline
Skew CVAR\\\hline
Kurtosis M\\\hline
Kurtosis STD\\\hline
Kurtosis CVAR\\\hline
Entropy M\\\hline
Entropy STD\\\hline
Entropy CVAR\\\hline
Median M\\\hline
Median STD\\\hline
Mutual information M\\\hline
Mutual information STD\\\hline
Mutual information CVAR\\\hline
Mutual information maximum value\\\hline
Correlation M\\\hline
Correlation STD\\\hline
Correlation CVAR\\\hline
Sparsity M\\\hline
Sparsity STD\\\hline
Sparsity CVAR\\\hline
Slice size M\\\hline
Slice size STD\\\hline
Slice size CVAR\\\hline
Number of slices M\\\hline
Number of slices STD \\\hline
Number of slices CVAR\\\hline
Equivalent number of features\\\hline
Noise signal ratio\\\hline
\end{tabular}}\\

\captionsetup{width=0.8\textwidth/2}
\caption{Statistical metafeatures used in the Support Vector Regression method. M = mean, STD = standard deviation, CVAR = coefficient of variation. }

\end{table}

\clearpage

\subsection{Full results SVR meta-learner}
Full results of SVR meta-learner. Consists of: MAE scores per MSD dataset, MAE scores per MSD challenge participant, method rank correlation and task rank correlation. 
\label{appendix:svrtot}
\setcounter{table}{0}

\begin{table}[htp]
\resizebox{\textwidth}{!}{%
\begin{tabular}{|ll|l|l|l|l|l|l|l|l|}
\hline
\multicolumn{2}{|c|}{\multirow{2}{*}{MSD datasets $\downarrow$}} & \multicolumn{8}{c|}{Mean absolute error $\downarrow$} \\ \cline{3-10} 
\multicolumn{2}{|c|}{} & \multicolumn{2}{c|}{Classical} & \multicolumn{2}{c|}{VGG16} & \multicolumn{2}{c|}{ResNet50} & \multicolumn{2}{c|}{MobileNetV1} \\ \cline{3-10} 
\multicolumn{2}{|l|}{Meta-learner $\rightarrow$} & \multicolumn{1}{c|}{SVR} & DNN & \multicolumn{1}{c|}{SVR} & DNN & \multicolumn{1}{c|}{SVR} & DNN & \multicolumn{1}{c|}{SVR} & DNN \\ \hline
1  & Braintumor     & $0.17\pm0.05$ & $0.06\pm0.06$ & $0.07\pm0.01$ & $0.09\pm0.01$ & $0.08\pm0.01$ & $0.22\pm0.06$ & $0.14\pm0.01$ & $0.22\pm0.06$ \\ \hline
2  & Heart          & $0.07\pm0.01$ & $0.18\pm0.05$ & $0.06\pm0.05$ & $0.09\pm0.01$ & $0.14\pm0.06$ & $0.05\pm0.01$ & $0.15\pm0.07$ & $0.11\pm0.02$ \\ \hline
3  & Liver          & $0.29\pm0.15$ & $0.55\pm0.25$ & $0.08\pm0.17$ & $0.03\pm0.00$ & $0.11\pm0.10$ & $0.04\pm0.00$ & $0.28\pm0.15$ & $0.24\pm0.06$ \\ \hline
4  & Hippocampus    & $0.07\pm0.01$ & $0.09\pm0.01$ & $0.04\pm0.07$ & $0.07\pm0.01$ & $0.08\pm0.07$ & $0.10\pm0.01$ & $0.06\pm0.07$ & $0.07\pm0.01$ \\ \hline
5  & Prostate       & $0.14\pm0.03$ & $0.27\pm0.09$ & $0.09\pm0.00$ & $0.21\pm0.05$ & $0.05\pm0.00$ & $0.07\pm0.01$ & $0.04\pm0.00$ & $0.05\pm0.01$ \\ \hline
6  & Lung           & $0.09\pm0.01$ & $0.09\pm0.01$ & $0.21\pm0.11$ & $0.23\pm0.06$ & $0.17\pm0.07$ & $0.10\pm0.02$ & $0.09\pm0.09$ & $0.09\pm0.02$ \\ \hline
7  & Pancreas       & $0.19\pm0.03$ & $0.07\pm0.01$ & $0.10\pm0.01$ & $0.09\pm0.01$ & $0.06\pm0.01$ & $0.09\pm0.01$ & $0.05\pm0.01$ & $0.16\pm0.04$ \\ \hline
8  & Hepatic vessel & $0.12\pm0.01$ & $0.10\pm0.05$ & $0.26\pm0.03$ & $0.21\pm0.06$ & $0.13\pm0.04$ & $0.21\pm0.05$ & $0.13\pm0.06$ & $0.09\pm0.02$ \\ \hline
9  & Spleen         & $0.46\pm0.18$ & $0.40\pm0.18$ & $0.08\pm0.14$ & $0.03\pm0.00$ & $0.10\pm0.11$ & $0.03\pm0.00$ & $0.21\pm0.10$ & $0.12\pm0.02$ \\ \hline
10 & Colon          & $0.54\pm0.23$ & $0.56\pm0.32$ & $0.31\pm0.28$ & $0.34\pm0.13$ & $0.31\pm0.25$ & $0.33\pm0.15$ & $0.36\pm0.30$ & $0.25\pm0.08$ \\ \hline
\textbf{} & \textbf{Total} & \multicolumn{1}{l|}{\textbf{$0.21\pm0.08$}} & \textbf{$0.24\pm0.09$} & \multicolumn{1}{l|}{\textbf{$0.13\pm0.09$}} & \textbf{$0.14\pm0.04$} & \multicolumn{1}{l|}{\textbf{$0.12\pm0.07$}} & \textbf{$0.12\pm0.03$} & \multicolumn{1}{l|}{\textbf{$0.15\pm0.09$}} & \textbf{$0.14\pm0.03$} \\ \hline
\end{tabular}%
}
\caption{Total MAE results of cross-validation on MSD datasets per dataset using a SVR meta-learner}
\label{tab:maetotmsvr}
\end{table}
\begin{table}[htp]
\resizebox{\textwidth}{!}{%
\begin{tabular}{|l|l|l|l|l|l|l|l|l|}
\hline
\multirow{2}{*}{Participants $\downarrow$} & \multicolumn{8}{c|}{Mean absolute error $\downarrow$} \\ \cline{2-9} 
 & \multicolumn{2}{c|}{Clasical} & \multicolumn{2}{c|}{VGG16} & \multicolumn{2}{c|}{ResNet50} & \multicolumn{2}{c|}{MobileNetV1} \\ \cline{2-9} 
Meta-learner $\rightarrow$ & SVR & DNN & SVR & DNN & SVR & DNN & SVR & DNN \\ \hline
Participant 1  & $0.25\pm0.08$ & $0.29\pm0.29$ & $0.08\pm0.11$ & $0.11\pm0.02$ & $0.18\pm0.10$ & $0.20\pm0.08$ & $0.19\pm0.12$ & $0.21\pm0.06$ \\ \hline
Participant 2  & $0.18\pm0.06$ & $0.19\pm0.19$ & $0.11\pm0.05$ & $0.11\pm0.02$ & $0.10\pm0.05$ & $0.12\pm0.03$ & $0.13\pm0.05$ & $0.13\pm0.02$ \\ \hline
Participant 3  & $0.20\pm0.05$ & $0.21\pm0.07$ & $0.12\pm0.06$ & $0.10\pm0.02$ & $0.11\pm0.05$ & $0.11\pm0.02$ & $0.13\pm0.06$ & $0.13\pm0.03$ \\ \hline
Participant 4  & $0.27\pm0.09$ & $0.24\pm0.10$ & $0.11\pm0.14$ & $0.14\pm0.03$ & $0.14\pm0.12$ & $0.17\pm0.04$ & $0.18\pm0.14$ & $0.13\pm0.03$ \\ \hline
Participant 5  & $0.19\pm0.70$ & $0.21\pm0.05$ & $0.12\pm0.06$ & $0.12\pm0.03$ & $0.11\pm0.05$ & $0.09\pm0.02$ & $0.12\pm0.06$ & $0.11\pm0.02$ \\ \hline
Participant 6  & $0.24\pm0.10$ & $0.25\pm0.11$ & $0.13\pm0.09$ & $0.15\pm0.03$ & $0.14\pm0.08$ & $0.11\pm0.02$ & $0.19\pm0.10$ & $0.18\pm0.04$ \\ \hline
Participant 7  & $0.21\pm0.07$ & $0.29\pm0.09$ & $0.16\pm0.12$ & $0.20\pm0.05$ & $0.15\pm0.09$ & $0.12\pm0.03$ & $0.15\pm0.11$ & $0.13\pm0.02$ \\ \hline
Participant 8  & $0.15\pm0.03$ & $0.16\pm0.02$ & $0.07\pm0.03$ & $0.07\pm0.01$ & $0.09\pm0.03$ & $0.07\pm0.01$ & $0.12\pm0.03$ & $0.11\pm0.02$ \\ \hline
Participant 9  & $0.24\pm0.10$ & $0.23\pm0.08$ & $0.14\pm0.08$ & $0.15\pm0.03$ & $0.12\pm0.07$ & $0.08\pm0.01$ & $0.22\pm0.08$ & $0.15\pm0.04$ \\ \hline
Participant 10 & $0.21\pm0.08$ & $0.27\pm0.10$ & $0.17\pm0.10$ & $0.19\pm0.06$ & $0.14\pm0.08$ & $0.16\pm0.06$ & $0.13\pm0.10$ & $0.12\pm0.02$ \\ \hline
Participant 11 & $0.24\pm0.09$ & $0.26\pm0.14$ & $0.17\pm0.09$ & $0.18\pm0.07$ & $0.14\pm0.08$ & $0.16\pm0.06$ & $0.15\pm0.1$  & $0.18\pm0.05$ \\ \hline
Participant 12 & $0.26\pm0.10$ & $0.26\pm0.15$ & $0.17\pm0.11$ & $0.20\pm0.06$ & $0.16\pm0.09$ & $0.16\pm0.04$ & $0.17\pm0.11$ & $0.15\pm0.04$ \\ \hline
Participant 13 & $0.18\pm0.06$ & $0.23\pm0.60$ & $0.11\pm0.06$ & $0.11\pm0.02$ & $0.01\pm0.05$ & $0.12\pm0.03$ & $0.14\pm0.06$ & $0.15\pm0.03$ \\ \hline
Participant 14 & $0.15\pm0.04$ & $0.18\pm0.03$ & $0.08\pm0.04$ & $0.09\pm0.01$ & $0.09\pm0.03$ & $0.08\pm0.01$ & $0.10\pm0.04$ & $0.10\pm0.02$ \\ \hline
Participant 15 & $0.17\pm0.04$ & $0.19\pm0.04$ & $0.09\pm0.05$ & $0.08\pm0.01$ & $0.10\pm0.04$ & $0.10\pm0.01$ & $0.12\pm0.05$ & $0.10\pm0.02$ \\ \hline
Participant 16 & $0.22\pm0.09$ & $0.26\pm0.12$ & $0.15\pm0.08$ & $0.14\pm0.04$ & $0.12\pm0.07$ & $0.12\pm0.03$ & $0.14\pm0.09$ & $0.13\pm0.03$ \\ \hline
Participant 17 & $0.20\pm0.08$ & $0.24\pm0.09$ & $0.13\pm0.08$ & $0.13\pm0.04$ & $0.12\pm0.07$ & $0.11\pm0.03$ & $0.14\pm0.08$ & $0.16\pm0.04$ \\ \hline
Participant 18 & $0.28\pm0.12$ & $0.31\pm0.15$ & $0.21\pm0.15$ & $0.25\pm0.07$ & $0.15\pm0.11$ & $0.22\pm0.07$ & $0.19\pm0.13$ & $0.22\pm0.06$ \\ \hline
Participant 19 & $0.22\pm0.08$ & $0.25\pm0.09$ & $0.16\pm0.09$ & $0.15\pm0.05$ & $0.12\pm0.08$ & $0.11\pm0.02$ & $0.14\pm0.09$ & $0.13\pm0.03$ \\ \hline
\textbf{Total} & \textbf{$0.21\pm0.08$} & \textbf{$0.24\pm0.10$} & \textbf{$0.13\pm0.09$} & \textbf{$0.14\pm0.04$} & \textbf{$0.13\pm0.07$} & \textbf{$0.13\pm0.03$} & \textbf{$0.15\pm0.09$} & \textbf{$0.14\pm0.03$} \\ \hline
\end{tabular}%
}
\caption{Total MAE results of cross-validation on MSD datasets per participant using a SVR meta-learner}
\label{tab:maetotsvr}
\end{table}
\clearpage
